# Supplementary material for: Assisting the Human Fact-Checkers: Detecting All Previously Fact-Checked Claims in a Document
Source: arXiv:2109.07410 source file (2022-11-15)
Supplement: Supplementary file 1 [file appendix.tex]

% \section{Dataset: More Details}
% In Table \ref{table:examples}, we provide a few examples of input sentence, verified claim with their stance and verdict label. 
% %It shows that whether input sentences agrees or disagrees with verified claim and the verdict. 

% For the data preparation of this study we followed several manual and automatic steps as 
% % For this study Dataset preparation process is 
% sketched in Figure~\ref{fig:data_prep_pipeline}.
% and described in more detail below. 
%Below, we describe the process in detail, as also shown in Figure \ref{fig:data_prep_pipeline}.


% \begin{figure}[h]
% \centering
% \includegraphics[width=0.47\textwidth]{figures/data_preparing_pipeline.png}
% \caption{Data preparation pipeline.}
% \label{fig:data_prep_pipeline}
% \end{figure}



% \subsection*{Statistics of the Dataset}
% In Table \ref{table:distribution}, we report the distribution of the PolitiFact dataset. 

% \begin{table}[h]
% \centering
% \scalebox{0.8}{
% \begin{tabular}{@{}lrr@{}}
% \toprule
% \multicolumn{1}{c}{\textbf{Politifact Truth   Value}} & \multicolumn{1}{c}{\textbf{True/False}} & \multicolumn{1}{c}{\textbf{Unknown}} \\ \midrule
% Pants on Fire! & 24 & 191 \\
% FALSE & 76 & 382 \\
% Mostly--False & 44 & 312 \\
% Half--True & 2 & 260 \\
% Mostly--True & 42 & 227 \\
% TRUE & 11 & 85 \\ \bottomrule
% \end{tabular}%
% }
% \caption{\textbf{Distribution:} \iclaim--\vclaim pairs with a true/false verdict vs. the \emph{TruthValue} for \vclaim claim from \politifact.}
% \label{table:distribution}
% \end{table}

% Table~\ref{table:transcript-stance-stats} reports some statistics about each transcript, as well as overall (last row). Shown are
% (\emph{i})~the number of sentences per transcript,
% (\emph{ii})~total number of sentences with top 15 verified claim pairs,
% (\emph{iii})~the number of input sentences for which there is a \vclaim claim with an \agree or a \disagree stance (column \emph{Stance-Input}),
% (\emph{iv})~the number of pairs with an \agree or a \disagree stance (column: \emph{Stance-pairs}),
% (\emph{v})~the number of input sentences for which there is a \emph{true}/\emph{false} verdict (column \emph{Verdict-Input}), and
% (\emph{vi})~the number of pairs with a \emph{true}/\emph{false} verdict (column: \emph{Verdict-pairs}).



% \todo{Have better examples}
% \begin{table*}[tbh!]
%     \centering
%     \small
%     \resizebox{1.0\textwidth}{!}{%
%     % \scalebox{0.88}{
%     \begin{tabular}{l  p{0.27\textwidth}  p{0.3\textwidth} p{0.17\textwidth}  l l}
%         \toprule
%         \bf No. & \bf \iclaim Sentence & \bf \vclaim Claim & \bf Label \& Date & \bf Stance & \bf Verdict \\
%         \midrule
%         % 1 & \emph{The stock market is in 22,000.} & {\bf Donald Trump:} The stock market has hit record numbers, as you know. And there has been a tremendous surge of optimism in the business world. & \textit{Mostly True}, stated on February 16, 2017 & Agree & True \\ \\
%         % 2 & \emph{The stock market is in 22,000.} & {\bf Jim Webb:} The stock market has almost tripled since April of 2009. & \textit{Mostly True}, stated on March 15, 2015 & Discuss & Unknown  \\ \\
%         % 1 & \emph{The reason why Democrats only talk about at the totally made up Russia story is because they have no message, no agenda, and no vision.} & \textbf{Donald Trump:} This Russia thing with Trump and Russia is a made-up story. It's an excuse by the Democrats for having lost an election that they should've won.   & \textit{Pants on Fire!}, stated on May 11, 2017 & \agree & False  \\ \\
%         1 & \emph{But the Democrats, by the way, are very weak on immigration.} & \textbf{Donald Trump:} The weak illegal immigration policies of the Obama Admin. allowed bad MS 13 gangs to form in cities across U.S. We are removing them fast!   & \textit{False}, stated on April 18, 2017 & \agree & Unknown  \\ \\
%         2 & \emph{ICE  we're getting MS13 out by the thousands.} & \textbf{Donald Trump:} Says of MS13 gang members, "We are getting them out of our country by the thousands."   & \textit{Mostly-False}, stated on May 15, 2018 & \agree & False  \\ \\
%         3 & \emph{ICE  we're getting MS13 out by the thousands.} & \textbf{Donald Trump:} I have watched ICE liberate towns from the grasp of MS13.  & \textit{False}, stated on June 30, 2018 & \agree & Unknown  \\ \\
% %        4 & \emph{While in the meantime the economy hit an all time high this morning.} & \textbf{Donald Trump:} Corporations have NEVER made as much money as they are making now.  & \textit{Half-True}, stated on August 1, 2017 & \agree & Unknown \\ \\
% %        5 & \emph{But we are going to get rid of Obamacare.} & \textbf{Ed MacDougall:} Says U.S. House candidate Carlos Curbelo "opposes the repeal of Obamacare."  & \textit{Mostly-False}, stated on July 26, 2014 & \disagree & Unknown \\ \\
%         4 & \emph{We have one of the highest business tax rates anywhere in the world, pushing jobs and wealth out of our country.} & \textbf{Barack Obama:} "There are so many loopholes ... our businesses pay effectively one of the lowest tax rates in the world."  & \textit{Half-True}, stated on September 26, 2008 & \disagree & Unknown \\
%         \bottomrule
%     \end{tabular}
%     }
%     \caption{Example sentences from Donald Trump's Interview with Fox and Friends on June 6th, 2018.}
%     \label{table:examples}
% \end{table*}


% \begin{table*}[tbh!]
% \centering
% \resizebox{1.0\textwidth}{!}{%
% % \scalebox{0.8}{
% % \setlength{\tabcolsep}{2.0pt}
% \begin{tabular}{@{}llrrrrrrr@{}}
% \toprule
% \multicolumn{1}{c}{\textbf{Date}} & \multicolumn{1}{c}{\textbf{Event}} & \multicolumn{1}{c}{\textbf{\# Topic}} & \multicolumn{1}{c}{\textbf{Sent.}} & \multicolumn{1}{c}{\textbf{Sent.-Var. Pairs}} & \multicolumn{1}{c}{\textbf{\# Stance-Input}} & \multicolumn{1}{c}{\textbf{\# Stance-pairs}} & \multicolumn{1}{c}{\textbf{\# Verdict-Input}} & \multicolumn{1}{c}{\textbf{\# Verdict-pairs}} \\ \midrule
% 2017-08-03 & Rally Speech & 3-4 & 291 & 4,365 & 34 & 62 & 20 & 32 \\
% 2017-08-22 & Rally Speech & 5+ & 792 & 11,880 & 50 & 116 & 23 & 40 \\
% 2018-04-26 & Interview & 5+ & 597 & 8,955 & 28 & 52 & 17 & 32 \\
% 2018-05-25 & Naval Grad. Speech & 1-2 & 279 & 4,185 & 14 & 19 & 4 & 5 \\
% 2018-06-12 & North Korea Summit Speech & 1-2 & 1,245 & 18,675 & 29 & 45 & 15 & 15 \\
% 2018-06-15 & Interview & 3-4 & 814 & 12,210 & 24 & 36 & 11 & 17 \\
% 2018-06-28 & Rally Speech & 5+ & 1,036 & 15,540 & 49 & 82 & 35 & 57 \\ \midrule
% \textbf{Total} &  & \multicolumn{1}{l}{} & 5,054 & 75,810 & 228 & 412 & 125 & 198 \\ \bottomrule
% \end{tabular}%
% }
% \caption{\textbf{Statistics about our dataset:} number of sentences in each transcript, and distribution of clear stance (\agree + \disagree) and clear verdict (true + false) labels. The number of topics were manually decided by looking at the keywords detected in each transcript. Sent.: number of input sentences, Sent.-Var. Pairs: number of input sentences with top 15 verified claims pairs.}
% \label{table:transcript-stance-stats}
% \end{table*}
